# Supplementary material for: FlexMoE: Scaling Large-scale Sparse Pre-trained Model Training via Dynamic Device Placement
Source: arXiv:2304.03946 source file (2023-04-08)
Supplement: Supplementary file 1 [file appendix.tex]

\newpage
\section{Appendix}

\begin{figure}[t]
\small
\begin{spacing}{0.8}
\begin{framed}
%\vspace{3mm}
\begin{align*}
\text{----~\textbf{Problem Formulation}~----}       
\end{align*}
\textit{\hspace{30pt} \textbf{Input}    \hspace{100pt}      \textbf{Output}}
%\vspace{-10pt}
\begin{align*}
& \text{- Experts } E:=E_{1\rightarrow n}
%, \left |L\right | = n
&& \text{- Device Placement } P:=P_{1\rightarrow g}\\
%, \left |B\right | = m\\
%& && \text{- Execution Stages } S_{1\rightarrow s}\\
%&\text{- Comp. cost: }Comp(l), l \in L && \text{- Exec. Schedule for B: } <B>\\ 
%&\text{- Mem cost:} Mem(l), l \in L \\
\end{align*}
\vspace{-20pt}
\textit{\textbf{Minimize}}
%\vspace{-20pt}
\begin{align}
\\
&\sum_{i=1}^{n}\left\{ Comp(B_{ij}) + 4*Transfer(B_{ij}) + Sync(E_{i}) \right\} + Migrate(\delta) \notag \\
&~~~~~~~~~~~~~~~~~~~~~~~~~~~~~~~~~~~ \forall  j \in  \{1,\ldots,g\}  \notag
\end{align}
\textit{\textbf{Subject to}} 
\begin{align}
&\sum_{j=1}^{g} \delta_{ij} \geq 1\text{~~~~~~~~~~~~~, }
\forall  i \in  \{1,\ldots,n\} \\
&\sum_{i=1}^{n} \delta_{ij} \leq K \text{~~~~~~~~~~~~~, }
\forall  j \in  \{1,\ldots,g\} \\
&\sum_{j=1}^{g} \delta_{ij}B_{ij} = B_{i} \text{~~~~~~~, }
\forall  i \in  \{1,\ldots,n\} \\
\end{align}
\vspace{-10pt}
\\\textit{\textbf{Where}}
%&y_{ab} = 1 \text{ if in the dependency graph of array } d_{l}\text{,}\\ 
%&\;\;\;\;\;\;\;\;\text{ kernel } k_{a} \text{ has a path to kernel } k_{b}
%&\delta_{ij} \in \left \{  0,1\right \}\text{~~~~~~~~~~~~~~~, }\forall i \in \left \{  1,\ldots,l\right \} \forall j \in \left \{  1,\ldots,b\right \}\\ 
\begin{align*}
&B_{i} ~~~~~~~~~~~~~~~~~~~~~~ \text{~Amount of tokens for i-th Expert} \\
&B_{ij} ~~~~~~~~~~~~~~~~~~~~~ \text{Amount of tokens for i-th Expert on j-th GPU} \\
&K ~~~~~~~~~~~~~~~~~~~~~~~\text{Total available expert replicas}\\
&\delta_{ij}^{t} \in \{0,1\} ~~~~~~~~ \delta_{ij}^{t}=1~\text{if i-th Expert} \text{~exits~in~j-th GPU at time}~t~ \\
% &\blue{\beta_{jj'} \in \{0,1\} ~~~~~~ \beta_{jj'}=1~\text{if j-th and j'-th GPU~exits~in~same~node}}~ \\
&Comp\left (  t\right ) ~~~~~~~~~~~\text{Fwd and bwd time for computing}~t~\text{token~} \\
&Transfer(B_{ij}) ~~~ \text{Return the j-th GPU' transfer time about B}_{i,j} \\
&Sync(E_{i}) ~~~~~~~~~~~~ \text{Return the sync time for i-th Expert} \\
&Migrate(\delta) ~~~~~~~~~~~~ \text{Return the migration time}
\end{align*}
\end{framed}
\end{spacing}
%\vspace{-5pt}
\caption{}
\end{figure}
